# Supplementary material for: Discovery-Targeted False Discovery Rate Control
Source: arXiv:2611.30031 source file (2026-11-23)
Supplement: Supplementary file 1 [file appendix-rows.tex]

% Generated by code/report_iterated_minimum.py; do not edit.
\begin{tabular}{@{}lrrr@{}}
\toprule
Metric & Proposal & One step & Iterated\\
\midrule
Reported $\widehat q_{50}$ & 0.088 & 0.142 & 0.127 \\
Rejections & 57.2 & 90.2 & 82.4 \\
$R\ge25$ (\%) & 88.2 (0.59) & 99.3 (0.16) & 98.4 (0.23) \\
\bottomrule
\end{tabular}
